# Supplementary material for: Non-equilibrium evolution of volatility in origination and extinction explains fat-tailed fluctuations in Phanerozoic biodiversity
Source: arXiv:1707.09268 ancillary file (2019-05-10)
Supplement: Supplementary file 1 [file appendix_a.pdf]

# Appendix A: R code to reproduce the study

The easiest way to reproduce this study is to download, clone, or fork the GitHub repository at `github.com/ajrominger/paleo_supStat`. All scripts can then be run on new downloads of the PBDB and modifications to the analyses can be made. The repository is organized into directories `data` containing data and data-cleaning scripts; `R` containing R functions for general use; and `analysis` containing analysis scripts that use the data and R functions. The GitHub repository also contains a manuscript directory (`ms`), this document (`sstat_notebook.Rmd`), and an R script (`sstat_make.R`) that calls each data cleaning and analysis script in sequence to automatically reproduce the entire study. The `data`, `R`, and `analysis` directories can also be recreated from the scripts reproduced below.

The accompanying explanations below (organized by the flow of data acquisition, cleaning, and then analysis) will help the user understand the purpose of each script/function such that they can reproduce the results, or modify the routine.

Lastly, this study depends on the contributed packages *divDyn*, *parallel*, and *R.utils* which should be installed from CRAN, and on a custom package *socorro* which must be installed from GitHub (using the *devtools* package):

```
devtools::install_github('ajrominger/socorro')
```

## A1 Getting the data

### A1.1 PBDB API

To obtain the PBDB data we make use of the API in script `data/pbdb_data_get.R`, which accesses the API and cleans the data by:

- removing poorly lithified specimens
- removing collections at the basin scale
- including only fine-scale stratigraphy (below the "group" level)
- resolving taxonomy to the genus or subgenus level where available (storing genus or subgenus as `otu`)
- combining multiple records of the same OTU per collection
- importing standardized time bins from fossilworks.org (time bins are scraped with script `data/fossilworks_tbins_intervals.R`)

The data gathering script `data/pbdb_data_get.R` is shown below:

```
# **script to interface with PBDB API and clean resulting data**

# call to the API
show <- paste0(c('ident', 'phylo', 'lith', 'loc', 'time', 'geo', 'stratext',
                 'ecospace'),
               collapse = ',')
version <- '1.2'
base_name <- 'Animalia^Craniata'
min_ma <- 0
max_ma <- 560
timerule <- 'contain'
envtype <- 'marine'

# break-up backbone URI just so it can be nicely displayed
bbURI <- paste0('https://paleobiodb.org/data%s/occs/list.csv?',
```

```r
                'base_name=%s&show=%s&limit=all&min_ma=%s&max_ma=%s&',
                'timerule=%s&envtype=%s')

# the actual call to the URI
uri <- sprintf(bbURI,
               version,
               base_name,
               show,
               min_ma,
               max_ma,
               timerule,
               envtype)

# get pbdb occurences
x <- read.csv(uri, as.is = TRUE)

# write out raw data
write.csv(x, 'data/pbdb_data_raw.csv', row.names = FALSE)


# clean up

# remove unnecceary columns
c2rm <- c('record_type', 'reid_no', 'flags', 'identified_name',
          'identified_rank', 'identified_no', 'difference', 'species_name',
          'species_reso', 'lithdescript', 'lithology1', 'minor_lithology1',
          'lithology2', 'lithification2', 'minor_lithology2', 'cc', 'state',
          'county', 'latlng_basis', 'geogcomments', 'geology_comments',
          'zone', 'localsection', 'localbed', 'localorder',
          'regionalsection', 'regionalbed', 'regionalorder',
          'stratcomments')
x <- x[, !(names(x) %in% c2rm)]

# only well lithified specimens
x <- x[x$lithification1 %in% c('', 'lithified'), ]


# no basin-scale collections
x <- x[x$geogscale != 'basin', ]

# fine scale stratigraphy only
x <- x[!(x$stratscale %in% c('group', 'supergroup')), ]

# resolve taxonomy to genus or subgenus where availible
otu <- x$genus
otu[x$subgenus_name != ''] <- ifelse(x$subgenus_reso[x$subgenus_name != ''] == '',
                                     x$subgenus_name[x$subgenus_name != ''],
                                     otu[x$subgenus_name != ''])
otu[x$primary_reso != ''] <- ''
x$otu <- otu
x <- x[x$otu != '', ]
```

```
# combine multiple records of same otu per collection
x <- x[!duplicated(x[, c('collection_no', 'otu')]), ]


# standard time bins
stages <- read.csv('data/tbins_stages.csv', as.is = TRUE)
earlyTbin <- stages$tbin[match(x$early_interval, stages$name)]
lateTbin <- stages$tbin[match(x$late_interval, stages$name)]
lateTbin[is.na(lateTbin)] <- earlyTbin[is.na(lateTbin)]
earlyTbin[earlyTbin != lateTbin] <- NA

x$tbin <- earlyTbin
x <- x[!is.na(x$tbin), ]


# write out fully processed data
write.csv(x, 'data/pbdb_data.csv', row.names = FALSE)
```

## A1.2 Scraping fossilworks

The script to pull Alory's time bins (`data/fossilworks_tbins_intervals.R`) is below:

```
# **script to scrape time bins from fossilworks.org**

options(stringsAsFactors = FALSE)

# loop through interval info on fossilworks.org
coreURI <- 'http://fossilworks.org/bridge.pl?a=displayInterval&interval_no='

tbinInfo <- lapply(1:1108, function(i) {
    print(i)
    linfo <- try(readLines(paste0(coreURI, i), n = 150))

    if('try-error' %in% class(linfo))
        linfo <- try(readLines(paste0(coreURI, i), n = 150))

    if('try-error' %in% class(linfo)) {
        thisTbin <- thisMax <- thisMin <- thisName <- NA
    } else {
        thisTbin <- gsub('^.*10 million year bin: |<br>.*$', '',
                         linfo[grep('10 million year bin', linfo)])
        thisMax <- as.numeric(gsub('^.*Lower boundary: equal to | Ma.*$|[^0-9\\.]', '',
                                   linfo[grep('Lower boundary: equal to', linfo)]))
        thisMin <- as.numeric(gsub('^.*Upper boundary: equal to | Ma.*$|[^0-9\\.]', '',
                                   linfo[grep('Upper boundary: equal to', linfo)]))
        thisName <- gsub('^.*<p class="pageTitle">|</p>.*$', '',
                         linfo[grep('class="pageTitle"', linfo)])
    }

    return(data.frame(name = ifelse(length(thisName) == 0, NA, thisName),
                      tbin = ifelse(length(thisTbin) == 0, NA, thisTbin),
                      ma_min = ifelse(length(thisMin) == 0, NA, thisMin),
                      ma_max = ifelse(length(thisMax) == 0, NA, thisMax)))
```

```r
})

tbinInfo <- do.call(rbind, tbinInfo)


# clean up
# --------

tbinInfo <- tbinInfo[!is.na(tbinInfo$name), ]

# remove 'stage' and equivilant from name
tbinInfo$name <- gsub(' [[:lower:]].*', '', tbinInfo$name)

# split up stages with a '/' into both names
temp <- tbinInfo[grep('/', tbinInfo$name), ]
tbinInfo$name <- gsub('.*/', '', tbinInfo$name)
temp$name <- gsub('/.* ', ' ', temp$name)
tbinInfo <- rbind(tbinInfo, temp)

# fix random typo
tbinInfo$name[tbinInfo$name == 'Cazenovia'] <- 'Cazenovian'


# write out
write.csv(tbinInfo, 'data/tbins_stages.csv', row.names = FALSE)


# also write out summary of each time bin, most importantly (for plottin)
# its midpoint

tbinmid <- sapply(unique(tbinInfo$tbin[!is.na(tbinInfo$tbin)]), function(tbin) {
    tt <- unlist(tbinInfo[tbinInfo$tbin == tbin, c('ma_min', 'ma_max')])
    return(mean(range(tt, na.rm = TRUE)))
})

tbinmid <- sort(tbinmid, decreasing = TRUE)

write.csv(data.frame(tbin = names(tbinmid), ma_mid = as.numeric(tbinmid)),
          'data/tbinsMid.csv', row.names = FALSE)


# lastly confirm the durations of tbins
length(tbinmid)

tbinrange <- sapply(unique(tbinInfo$tbin[!is.na(tbinInfo$tbin)]), function(tbin) {
    tt <- unlist(tbinInfo[tbinInfo$tbin == tbin, c('ma_min', 'ma_max')])
    return(diff(range(tt, na.rm = TRUE)))
})

mean(tbinrange)
```

## A2 Three timer and publication bias correction

Once the data have been downloaded and cleaned, we correct for incomplete and biased sampling with the script `data/pbdb_3TPub_make.R` which sources the function `R/make3TPub.R` to generate the main output: a matrix with time bins as rows, taxa (families in this case) as columns and bias-corrected richness as cells.

```
# **this script produces diversity estimates per family per time bin from PBDB data
# corrected by the '3 timers method' and for possible publication bias**

# source function to produce a matrix of time by taxon with cells
# of corrected diversity
source('R/make3TPub.R')

# load other needed funcitons

# source('code/sstat_comp.R')
# source('code/sstat_methods.R')
# source('code/Px_gam.R')

# load and prepare data
# ---------------------

pbdbDat <- read.csv('data/pbdb_data.csv', as.is = TRUE)

# make column for midpoint ma
pbdbDat$ma_mid <- (pbdbDat$max_ma + pbdbDat$min_ma) / 2

# get rid of poor temporal resolution
pbdbDat <- pbdbDat[pbdbDat$tbin != '', ]

# get rid of bad taxonomy
pbdbDat <- pbdbDat[pbdbDat$family != '', ]
pbdbDat <- pbdbDat[pbdbDat$otu != '', ]

# get bin times
pbdbDat$mid_ma <- (pbdbDat$min_ma + pbdbDat$max_ma) / 2
pbdbTime <- sort(tapply(pbdbDat$mid_ma, pbdbDat$tbin, mean))
pbdbDat$tbin <- factor(pbdbDat$tbin, levels = names(pbdbTime))


# data.frame to hold publication, diversity and 3T stat
famTbinBias <- aggregate(list(div = pbdbDat$otu), list(fam = pbdbDat$family,
                                                       tbin = pbdbDat$tbin),
                         function(x) length(unique(x)))


# three timer stat and publication bias
# -------------------------------------

# matrix to determine three timers and part timers (sensu alroy 2008)
mt <- matrix(0, nrow = nlevels(pbdbDat$tbin),
             ncol = nlevels(pbdbDat$tbin))
diag(mt) <- -10
mt[abs(row(mt) - col(mt)) == 1] <- 1
```

```r
# loop through and compute three timers and part timers
timers <- lapply(split(pbdbDat$tbin, pbdbDat$otu),
                 function(x) {
                     # browser()
                     tbins <- integer(nlevels(x))
                     tbins[as.integer(unique(x))] <- 1
                     t3 <- as.integer(mt %*% tbins == 2)
                     tp <- as.integer(mt %*% tbins == -8)

                     return(cbind(t3, tp))
                 })

# compute 3 timer stat from 3 timers and part timers
timers <- array(unlist(timers), dim = c(nrow(timers[[1]]), 2, length(timers)))
t3stat <- 1 - rowSums(timers[, 1, ]) / (rowSums(timers[, 1, ]) + rowSums(timers[, 2, ]))

# add to data.frame holding all info to be saved
famTbinBias$T3Stat <- t3stat[match(famTbinBias$tbin,
                                   levels(pbdbDat$tbin))]
famTbinBias$T3Div <- famTbinBias$div / famTbinBias$T3Stat

# record pubs per tbin
tbinPub <- tapply(pbdbDat$reference_no, pbdbDat$tbin,
                  function(x) length(unique(x)))
famTbinBias$tbinPub <- tbinPub[famTbinBias$tbin]

# calculate corrected diversity
pdf('ms/figSupp_divByPub_foo.pdf', width = 4, height = 4)
pbdbFamDiv <- with(famTbinBias,
                   make3TPub(div, T3Stat, tbinPub, fam, tbin, pbdbTime,
                             minPub = 10, plotit = TRUE))
dev.off()

# write out corrected diversity
write.csv(pbdbFamDiv, 'data/pbdb_3TPub-corrected.csv')


# for permutational d-stat tests we need diversity at the genus level;
# make that here

# a data.frame holding only one record per genus per family per time bin
pbdbOcc <- pbdbDat[!duplicated(pbdbDat[, c('tbin', 'family', 'otu')]), ]

genTbinBias <- parallel::mclapply(which(!is.nan(famTbinBias$T3Stat)), mc.cores = 3,
                                  FUN = function(i) {
                                      dat <- pbdbOcc[pbdbOcc$family == famTbinBias$fam[i] &
                                                         pbdbOcc$tbin == famTbinBias$tbin[i],
                                                     c('tbin', 'family', 'otu')]
                                      dat$T3Occ <- 1 / famTbinBias$T3Stat[i]
                                      dat$tbinPub <- famTbinBias$tbinPub[i]

                                      return(dat)
                                  }
```

```r
)

genTbinBias <- do.call(rbind, genTbinBias)
pbdbGenDiv <- data.frame(genTbinBias[, c('tbin', 'family', 'otu')],
                         T3PubDiv = genTbinBias$T3Occ /
                             exp(predict(pbdbPubLM,
                                         newdata = data.frame(
                                             logPub = log(genTbinBias$tbinPub)))))

# write it out as a tidy data frame (not turned into a matrix) this will be easier
# for permuting
write.csv(pbdbGenDiv, file = 'data/pbdb_3TPub_genera.csv', row.names = FALSE)
```

Here is the guts of the `make3TPub` function

```r
#' @description function to produce a matrix of time by taxa with cells of corrected diversity
#' @param rawDiv the raw diversity of each taxon in each time interval
#' @param t3stat the 3 timer stat for each diversity record
#' @param pub the number of publications associated with each diversity record
#' @param taxa the taxon names for each diversity record
#' @param tbin the time interval of each diversity record
#' @param tbinTime times associated with each `tbin`
#' @param minPub minimum number of publications for inclusion in regression analysis
#' @param plotit logical, should plot of taxon richness versus number of publications be made
#' @return a matrix with rows corresponding to time intervals and columns to the given taxa
#' each cell in the matrix represents corrected taxon richness


make3TPub <- function(rawDiv,  t3stat,  pub,  taxa,  tbin,  tbinTime,
                      minPub = 10,  plotit = FALSE) {
    # put data together so can be universally manipulated
    x <- data.frame(rawDiv = rawDiv, t3stat = t3stat, pub = pub, taxa = taxa, tbin = tbin)
    x$tbin <- as.character(x$tbin)
    x$taxa <- as.character(x$taxa)

    x <- x[!is.na(t3stat) & pub >=  minPub, ]

    tbinTime <- tbinTime[names(tbinTime) %in% x$tbin]

    # 3-timer correction
    t3cor <- x$rawDiv/x$t3stat

    # publication correction
    logPub <- log(x$pub)
    publM <- lm(log(t3cor)~logPub)
    pbdbPubLM <<- publM # save regression to global env

    pubResid <- exp(publM$residuals)

    # plot so you can verify cuttoff etc.
    if(plotit) {
        plot(log(x$pub), log(t3cor),
             xlab = 'log(Number of publications)',
             ylab = 'log(3T-corrected number of genera)')
```

```
        abline(pubLM, col = 'red')
    }

    tbinTaxa <- socorro::tidy2mat(x$tbin, x$taxa, pubResid)

    return(tbinTaxa[names(sort(tbinTime, decreasing = TRUE)), ])
}
```

Our publication correction is simple: we take the exponential of the residual of this relationship:

$$\log(\text{3T-corrected richness}) = \beta_0 + \beta_1 \log(\text{number of publications}) + \epsilon$$

The exponentiated residual amounts to dividing the three-timer corrected richness by a publication correction factor: (3T-corrected richness)$/e^{\hat{y}}$ where $\hat{y}$ is the predicted trend line from the above relationship.

So we can use this multiplicative publication correction factor in addition to the similarly multiplicative three-timer correction to bias-correct individual genus-level occurrences. This is important when we permute these bias-corrected genera across families to create a null set of d-statistics for our superstatistical fit.

We can check our correction against other popular methods. In the script `analysis/pbdb_divCurve.R` we specifically compare simple rarefaction, with the SQS method, with our three-time and publication bias correction methods. All these various methods have close agreement. The script `analysis/pbdb_divCurve.R` is shown below:

```
# **a script to compare our 3TPub curve to other estimates of richness through
# the Phanerozoic**

# package with diversity dynamics subsampling functions
library(divDyn)

# package for plotting
library(socorro)

# load and prep data
pbdbFamDiv <- read.csv('data/pbdb_3TPub-corrected.csv', row.names = 1)
pbdbDat <- read.csv('data/pbdb_data.csv', as.is = TRUE)
tbin <- read.csv('data/tbinsMid.csv', as.is = TRUE)
tbin$tbin <- factor(tbin$tbin, levels = tbin$tbin)
pbdbDat$tbin <- factor(pbdbDat$tbin, levels = levels(tbin$tbin))
pbdbDat$tbinNum <- as.integer(pbdbDat$tbin)

pbdbDatUnique <- pbdbDat[!duplicated(paste0(pbdbDat$collection_no, pbdbDat$otu)), ]

# subsampled richness
pbdbCR <- subsample(pbdbDatUnique, bin = 'tbinNum', tax = 'otu', iter = 50, q = 120,
                    type = 'cr', unit = 'reference_no')
pbdbSQS <- subsample(pbdbDatUnique, bin = 'tbinNum', tax = 'otu', iter = 50, q = 0.75,
                     ref = 'reference_no', type = 'sqs', singleton = 'ref')

# our new richness estimate
pbdbT3Pub <- rowSums(pbdbFamDiv)


# plot fluctuations to see that they're comprable
pdf('ms/figSupp_divEstComp.pdf', width = 8, height = 4)
layout(matrix(1:2, nrow = 1))
```

```r
par(mar = c(4.5, 2.5, 0, 0.5) + 0.5, mgp = c(2, 0.75, 0))
plot(1, xlim = c(540, 0), ylim = c(-400, 400), type = 'n', xaxt = 'n',
     xlab = '', ylab = 'Richness fluctuations', xaxs = 'i')
paleoAxis(1)
mtext('Millions of years ago', side = 1, line = 3.5)

lines(tbin$ma_mid[-1], diff(pbdbCR$divCSIB), col = 'black', lwd = 2)
lines(tbin$ma_mid[-1], diff(pbdbSQS$divCSIB), col = 'blue', lwd = 2)
lines(tbin$ma_mid[-c(1:2, nrow(tbin))], diff(pbdbT3Pub), col = 'red', lwd = 2)


par(mar = c(3, 3, 0, 0) + 0.5, mgp = c(2, 0.75, 0))
plot(simpECDF(c(1, abs(diff(pbdbT3Pub))), complement = TRUE), col = 'red', log = 'xy',
     type = 'l', lwd = 2, xlim = c(1, 500),
     panel.first = {
         lines(simpECDF(c(1, abs(diff(pbdbCR$divCSIB))), complement = TRUE),
               col = 'black', lwd = 2)
         lines(simpECDF(c(1, abs(diff(pbdbSQS$divCSIB))), complement = TRUE),
               col = 'blue', lwd = 2)
     },
     axes = FALSE, frame.plot = TRUE,
     xlab = '|Fluctuations|', ylab = 'Cumulative density')
logAxis(1:2)


legend('bottomleft', legend = c('Rarefaction', 'SQS', '3 timer pub'),
       lty = 1, lwd = 2, col = c('black', 'blue', 'red'), bty = 'n')

dev.off()
```

## A3 Super statistical analysis of 3TPub-corrected PBDB data

Once data have been bias-corrected we can complete their super-statistical analysis. We do that in the script `analysis/pbdb_sstat.R` shown here:

```r
# **script to run super stat analysis on PBDB data and make plots**

# source needed functions
R.utils::sourceDirectory('R', modifiedOnly = FALSE)
library(socorro) # for plotting

# load and prepare data
# ----------------------

pbdbFamDiv <- read.csv('data/pbdb_3TPub-corrected.csv', row.names = 1)


# coarsen to higher taxonomic groupings

pbdbTax <- read.csv('data/pbdb_taxa.csv', as.is = TRUE)

#' helper function to coarsen taxonomic resolution of `pbdbFamDiv` object
```

```r
#' @param level a character string specifying the taxonomic level (from order through phylum)

coarsenTaxa <- function(level) {
    m <- tidy2mat(pbdbTax$family[match(colnames(pbdbFamDiv), pbdbTax$family)],
                  pbdbTax[match(colnames(pbdbFamDiv), pbdbTax$family), level],
                  rep(1, ncol(pbdbFamDiv)))
    m <- m[colnames(pbdbFamDiv), ]

    out <- as.matrix(pbdbFamDiv) %*% m
    out <- out[, colnames(out) != '']

    return(out)
}

pbdbOrdDiv <- coarsenTaxa('order')
pbdbClsDiv <- coarsenTaxa('class')
pbdbPhyDiv <- coarsenTaxa('phylum')


# tbin midpoints
tbinMid <- read.csv('data/tbinsMid.csv', as.is = TRUE)
tbinNames <- tbinMid$tbin
tbinMid <- as.numeric(tbinMid[, 2])
names(tbinMid) <- tbinNames

tbinMid <- tbinMid[rownames(pbdbFamDiv)]


# super stat analysis
# -------------------


# calculate flux for families
pbdbFamFlux <- calcFlux(pbdbFamDiv)

# calculate the mean flux
famMeans <- sapply(pbdbFamFlux, mean)
mean(famMeans)
sd(famMeans)


# make sstat object for families
sstatPBDBfam3TP <- sstatComp(pbdbFamFlux, minN = 10, plotit = FALSE)

# deltaAIC
logLik(sstatPBDBfam3TP) - sum(dnorm(unlist(sstatPBDBfam3TP$Px.sub), log = TRUE))

# likelihood CI for family-level sstat analysis
sstatPBDBfam3TPCI <- bootMLE.sstat(sstatPBDBfam3TP, B = 1000, useAll = FALSE)


# do the same for higher taxo levels
pbdbOrdFlux <- calcFlux(pbdbOrdDiv)
```

```r
sstatPBDBOrd <- sstatComp(pbdbOrdFlux, minN = 10, plotit = FALSE)

# likelihood CI for family-level sstat analysis
sstatPBDBOrd3TPCI <- bootMLE.sstat(sstatPBDBOrd, B = 1000, useAll = FALSE)

pbdbClsFlux <- calcFlux(pbdbClsDiv)
sstatPBDBCls <- sstatComp(pbdbClsFlux, minN = 10, plotit = FALSE)

pbdbPhyFlux <- calcFlux(pbdbPhyDiv)
sstatPBDBPhy <- sstatComp(pbdbPhyFlux, minN = 10, plotit = FALSE)

# save the sstat analyses for future use
save(sstatPBDBfam3TP, sstatPBDBOrd, sstatPBDBCls, sstatPBDBPhy,
     file = 'data/pbdb_sstat_objects.RData')


# plot all sstat analyses
pdf('ms/fig_Px.pdf', width = 4.25 * 1.25, height = 4 * 1.25)

layout(matrix(1:4, nrow = 2, byrow = TRUE))
par(oma = c(3, 3, 0, 0) + 0.5, mar = c(0.1, 0.1, 1.51, 0.1),
    mgp = c(2, 0.5, 0), cex.lab = 1.4)

plot(sstatPBDBfam3TP, xlim = c(1e-04, 5e+02), ylim = c(8e-05, 1),
     xaxt = 'n', yaxt = 'n',
     panel.first = quote(mlePoly(sstatPBDBfam3TPCI$sstat, PPx.gam,
                                 col = hsv(alpha = 0.25), border = NA)))
mtext('Families', side = 3, line = 0)
logAxis(2, expLab = TRUE)
legend('topright', legend = 'A', bty = 'n', cex = 1.4)

plot(sstatPBDBOrd, xlim = c(1e-04, 5e+02), ylim = c(8e-05, 1), xaxt = 'n', yaxt = 'n',
     addLegend = FALSE,
     panel.first = quote(mlePoly(sstatPBDBOrd3TPCI$sstat, PPx.gam,
                                 col = hsv(alpha = 0.25), border = NA)))
mtext('Orders', side = 3, line = 0)
legend('topright', legend = 'B', bty = 'n', cex = 1.4)

plot(sstatPBDBCls, xlim = c(1e-04, 5e+02), ylim = c(8e-05, 1), xaxt = 'n', yaxt = 'n',
     addLegend = FALSE)
mtext('Classes', side = 3, line = 0)
logAxis(1:2, expLab = TRUE)
legend('topright', legend = 'C', bty = 'n', cex = 1.4)

plot(sstatPBDBPhy, xlim = c(1e-04, 5e+02), ylim = c(8e-05, 1), xaxt = 'n', yaxt = 'n',
     addLegend = FALSE)
mtext('Phyla', side = 3, line = 0)
logAxis(1, expLab = TRUE)
legend('topright', legend = 'D', bty = 'n', cex = 1.4)

mtext('|Fluctuations|', side = 1, outer = TRUE, line = 2)
mtext('Cumulative density', side = 2, outer = TRUE, line = 2)
```

```r
dev.off()




# plot p_k(x|b) and f(beta) for families
# --------------------------------------


# highlight individual trajectories
loFam <- 'Tainoceratidae' # nautiloid
miFam <- 'Lophospiridae' # sea snails
hiFam <- 'Spondylidae' # bivalve
lo <- pbdbFamDiv[, loFam]
mi <- pbdbFamDiv[, miFam]
hi <- pbdbFamDiv[, hiFam]
cols <- hsv(h = c(0.7, 0.45, 0.12), s = c(0.7, 1, 1), v = c(0.8, 0.8, 1))
names(cols) <- c('hi', 'mi', 'lo')

# make CDF for all scale family-level fluctuations
pAll <- lapply(sstatPBDBfam3TP$raw.pk,
               function(x) simpECDF(scale(x)[, 1], complement = TRUE))

pHighlight <- pAll[c(loFam, miFam, hiFam)]

pAll <- do.call(rbind, pAll)

# function to help with individual trajectory plotting
trajLines <- function(t, x, ...) {
    x[x == 0] <- NA
    alive <- range(which(!is.na(x)))

    x[min(alive) - 1] <- 0
    x[max(alive) + 1] <- 0

    t <- t[!is.na(x)]
    x <- x[!is.na(x)]

    lines(t, x, ...)
}

# the actual plotting

pdf('ms/fig_pkx-fbeta.pdf', width = 4.25 * 1.25, height = 4 * 1.25)

layout(matrix(c(1, 2, 1, 3), nrow = 2))

par(oma = c(0, 3, 0, 0) + 0.25, mar = c(4, 0, 0, 0) + 0.25,
    mgp = c(2, 0.5, 0), cex.lab = 1.4)

plot(1, xlim = c(540, 0), xaxt = 'n', xaxs = 'i', xlab = '',
     ylim = c(0, max(lo, mi, hi, na.rm = TRUE)), type = 'n')
```

```
trajLines(tbinMid, lo, col = cols['lo'], lwd = 2)
trajLines(tbinMid, mi, col = cols['mi'], lwd = 2)
trajLines(tbinMid, hi, col = cols['hi'], lwd = 2)

text(c(420, 230, 10), c(4, 5.25, 2), labels = c(miFam, loFam, hiFam),
     col = cols[c('mi', 'lo', 'hi')], pos = c(3, 4, 2))

paleoAxis(1)
mtext('Millions of years ago', side = 1, line = 3.5)
mtext('Standardized richness', side = 2, line = 2)

legend('topright', legend = 'A', pch = NA, bty = 'n', cex = 1.4)

# scale fluctuations
par(mar = c(3, 0, 1, 0) + 0.25)
plot(pAll, xlim = c(-4, 4), col = 'gray', ylim = c(0, 1.025),
     xlab = 'Scaled fluctuations')
mtext('Cumultive density', side = 2, line = 2)

for(i in 1:length(pHighlight)) lines(pHighlight[[i]], col = cols[i], lwd = 2)

curve(pnorm(x, lower.tail = FALSE), lwd = 2, add = TRUE)

legend('topright', legend = 'B', pch = NA, bty = 'n', cex = 1.4)

# CDF of beta
betaCDF <- simpECDF(sstatPBDBfam3TP$beta, complement = TRUE)
plot(betaCDF, ylim = c(0, 1.025),
     log = 'x', xaxt = 'n', yaxt = 'n',
     xlab = expression(beta), col = 'gray')

logAxis(1, expLab = TRUE)

curve(pgamma(x, sstatPBDBfam3TP$gam.par[1], sstatPBDBfam3TP$gam.par[2],
             lower.tail = FALSE),
      col = 'black', lwd = 2, add = TRUE)

theseBeta <- sstatPBDBfam3TP$beta[c(loFam, miFam, hiFam)]
points(theseBeta, approxfun(betaCDF)(theseBeta), bg = cols, pch = 21, cex = 1.2)


legend('topright', legend = 'C', pch = NA, bty = 'n', cex = 1.4)

dev.off()
```

Now we can calculate a measure of goodness of fit with the Kolmogorov-Smirnov test statistics $D$. That is done in the script `analysis/pbdb_dperm.R`. This script uses a permutation approach to create a null distribution of test statistics. The goal is to see if the good fit of super-statistics at the family and order levels is purely from the number of different groupings at those levels, regardless of the biology that might be going on to make those levels actually mechanistically meaningful. So to achieve such a null, we permute orders across families, calculate the D-statistics of those permuted groupings, and compare to the real D-statistics from the actual biological groupings. The script is shown below:

```r
# **script to caculate d stats on sstat objects and null permutations**

library(socorro)
R.utils::sourceDirectory('R', modifiedOnly = FALSE)

# read in data
pbdbGenDiv <- read.csv('data/pbdb_3TPub_genera.csv', as.is = TRUE)
pbdbTax <- read.csv('data/pbdb_taxa.csv', as.is = TRUE)
# pbdbFamDiv <- read.csv('data/pbdb_3TPub-corrected.csv', row.names = 1)
load('data/pbdb_sstat_objects.RData')

# the indeces of otu names in `pbdbTax` ordered by their occurence in `pbdbGenDiv`
# needed to match permuted families to genera
genHash <- match(pbdbGenDiv$otu, pbdbTax$otu)


#' function to calculate KS test d-stat on sstat objects
#' @param x an sstat object

ks.sstat <- function(x) {
    dat <- unlist(x$Px.sub)
    dat <- abs(dat)

    # cumulative density function
    pfun <- function(X) x$PPx(X, comp = TRUE)

    # cumulative prob observed and from theory
    n <- length(dat)
    pobs <- (n:1) / n
    pthr <- pfun(sort(dat))

    # the statisic is the difference between obs and thr
    out <- pthr - pobs

    return(max(out, 1 / n - out, na.rm = TRUE))
}


# sstat on real (non-permuted) data
dObsFam <- ks.sstat(sstatPBDBfam3TP)
dObsOrd <- ks.sstat(sstatPBDBOrd)
dObsCls <- ks.sstat(sstatPBDBCls)
dObsPhy <- ks.sstat(sstatPBDBPhy)


# repeatedly permute data and calculate null ks statistics
B <- 500
dNull <- parallel::mclapply(1:B, mc.cores = 8, FUN = function(i) {
    newFam <- sample(pbdbTax$family)
    newDiv <- tidy2mat(pbdbGenDiv$tbin, newFam[genHash], pbdbGenDiv$T3PubDiv)
    newFlux <- calcFlux(newDiv)
    newSstat <- sstatComp(newFlux, minN = 10, plotit = FALSE)
```

```r
    ks.sstat(newSstat)
    # return(ks.sstat(newSstat))
})

dNull <- unlist(dNull)


# save output in case it's ever needed
save(dNull, file = 'data/dnull.RData')


# plotting
pdf('ms/fig_dStat.pdf', width = 4, height = 4)
# colors for plotting taxa
tcols <- colorRampPalette(hsv(c(0.12, 0, 0.02), c(1, 0.9, 0.7), c(1, 0.8, 0.3)))(4)

par(mar = c(3, 3, 0, 0) + 0.5, mgp = c(2, 0.75, 0))
denFill(dNull, xlim = range(dNull, dObsFam, dObsOrd, dObsCls, dObsPhy) * c(0.9, 1.1),
        xlab = 'D-statistic', main = '')

abline(v = dObsFam, lwd = 2, col = tcols[1])
text(dObsFam, 1.25 * mean(par('usr')[3:4]), labels = 'Families', col = tcols[1],
     srt = 90, pos = 4)

abline(v = dObsOrd, lwd = 2, col = tcols[2])
text(dObsOrd, 1.25 * mean(par('usr')[3:4]), labels = 'Orders', col = tcols[2],
     srt = 90, pos = 4)

abline(v = dObsCls, lwd = 2, col = tcols[3])
text(dObsCls, 1.25 * mean(par('usr')[3:4]), labels = 'Classes', col = tcols[3],
     srt = 90, pos = 4)

abline(v = dObsPhy, lwd = 2, col = tcols[4])
text(dObsPhy, 1.25 * mean(par('usr')[3:4]), labels = 'Phyla', col = tcols[4],
     srt = 90, adj = c(0, -0.5))

dev.off()
```

This permutation null test is in part motivated by the correlation between the genus richness of a family and its $\beta_k$ value. We demonstrate this correlation in the script `analysis/pbdb_betaRichness.R` which is reproduced below:

```r
library(socorro)

load('data/pbdb_sstat_objects.RData')
pbdbDat <- read.csv('data/pbdb_data.csv', as.is = TRUE)

divFamRaw <- tapply(pbdbDat$otu, pbdbDat$family, function(x) length(unique(x)))

pdf('ms/figSupp_betaByRich.pdf', width = 4, height = 4)
par(mar = c(3, 3, 0, 0) + 0.5, mgp = c(2, 0.75, 0))
plot(divFamRaw[names(sstatPBDBfam3TP$beta)], sstatPBDBfam3TP$beta, log = 'xy',
     xlab = 'Number of genera', ylab = expression(beta),
     axes = FALSE, frame.plot = TRUE)
```

```r
logAxis(1:2)
dev.off()
```

Now that we are reasonably convinced that these superstatistical findings are not just an artifact of taxonomy or clade size, we can explore why we see deviations from super statistics with increasing taxonomic level. We first explore how well the Gaussian $p_k(x|\beta_k)$ fit at each taxonomic level in the script `analysis/pkx_diffK.R` shown here:

```r
# **script to compare within clade fluctuation distributions at different taxonomic levels**

library(socorro)

# source needed functions
R.utils::sourceDirectory('R', modifiedOnly = FALSE)

load('data/pbdb_sstat_objects.RData')


# for each family, calculate aggregated eCDF and distribution of kurtosis values
famECDF <- lapply(sstatPBDBfam3TP$Px.sub, function(x) {
    simpECDF(scale(x)[, 1], complement = TRUE)
})
famECDF <- do.call(rbind, famECDF)
famKurt <- sapply(sstatPBDBfam3TP$Px.sub, kurt)

ordECDF <- lapply(sstatPBDBOrd$Px.sub, function(x) {
    simpECDF(scale(x)[, 1], complement = TRUE)
})
ordECDF <- do.call(rbind, ordECDF)
ordKurt <- sapply(sstatPBDBOrd$Px.sub, kurt)

clsECDF <- lapply(sstatPBDBCls$Px.sub, function(x) {
    simpECDF(scale(x)[, 1], complement = TRUE)
})
clsECDF <- do.call(rbind, clsECDF)
clsKurt <- sapply(sstatPBDBCls$Px.sub, kurt)

phyECDF <- lapply(sstatPBDBPhy$Px.sub, function(x) {
    simpECDF(scale(x)[, 1], complement = TRUE)
})
phyECDF <- do.call(rbind, phyECDF)
phyKurt <- sapply(sstatPBDBPhy$Px.sub, kurt)


#' @description function to plot theoretical and observed percentiles
#' @param x aggregated eCDF
#' @param ... additional plotting parameters

ppECDF <- function(x, ...) {
    alpha <- 0.75 / (1 + exp(0.0003 * (nrow(x) - 300))) # nicely scale transparency
    plot(pnorm(x[, 1], lower.tail = FALSE), x[, 2], pch = 16,
         col = gray(0, alpha = alpha), xlim = 0:1, ylim = 0:1, ...)

    abline(0, 1, col = 'red')
```

```r
}


#' @description function to plot summary of kurtosis values distribution
#' @param x kurtosis values
#' @param ... additional plotting parameters

kurtInset <- function(x, ...) {
    allMean <- c(mean(famKurt), mean(ordKurt), mean(clsKurt), mean(phyKurt))
    allSD <- c(sd(famKurt), sd(ordKurt), sd(clsKurt), sd(phyKurt))

    plot(1, mean(x), pch = 16,
         ylim = range(allMean - allSD, allMean + allSD) * c(1.5, 1.25),
         xaxt = 'n', frame.plot = FALSE, yaxs = 'i',
         ...)
    segments(x0 = 1, y0 = mean(x) - sd(x), y1 = mean(x) + sd(x))
}




# plot it
pdf('ms/figSupp_pkx_allTaxa.pdf', width = 9, height = 3)

split.screen(c(1, 4))

# first plots of the ECDF's
screen(1, new = FALSE)
par(mar = c(0.3, 0.3, 1.5, 0.3), oma = c(2.5, 2.5, 0, 0),
    mgp = c(2, 0.5, 0))
ppECDF(famECDF)
mtext('Families', side = 3, line = 0.5)

screen(2, new = FALSE)
par(mar = c(0.3, 0.3, 1.5, 0.3), oma = c(2.5, 2.5, 0, 0),
    mgp = c(2, 0.5, 0))
ppECDF(ordECDF, yaxt = 'n')
mtext('Orders', side = 3, line = 0.5)

screen(3, new = FALSE)
par(mar = c(0.3, 0.3, 1.5, 0.3), oma = c(2.5, 2.5, 0, 0),
    mgp = c(2, 0.5, 0))
ppECDF(clsECDF, yaxt = 'n')
mtext('Classes', side = 3, line = 0.5)

screen(4, new = FALSE)
par(mar = c(0.3, 0.3, 1.5, 0.3), oma = c(2.5, 2.5, 0, 0),
    mgp = c(2, 0.5, 0))
ppECDF(phyECDF, yaxt = 'n')
mtext('Phyla', side = 3, line = 0.5)


mtext('N(0, 1) percentiles', side = 1, outer = TRUE, line = 1.25)
```

```r
mtext('Observed percentiles', side = 2, outer = TRUE, line = 1.25)

close.screen(all.screens = TRUE)


# now inset plots of kurtosis

start <- 1/4 + 0.01
swidth <- 1/32
increment <- 1/4 - 1/64
s <- split.screen(matrix(c(start + 0 * increment, start + 0 * increment + swidth, 0.25, 0.6,
                           start + 1 * increment, start + 1 * increment + swidth, 0.25, 0.6,
                           start + 2 * increment, start + 2 * increment + swidth, 0.25, 0.6,
                           start + 3 * increment, start + 3 * increment + swidth, 0.25, 0.6),
                         ncol = 4, byrow = TRUE), erase = FALSE)

for(i in 1:4) {
    screen(s[i], new = FALSE)
    par(mar = rep(0, 4), mgp = c(1, 0.25, 0))
    kurtInset(switch(i,
                     `1` = famKurt,
                     `2` = ordKurt,
                     `3` = clsKurt,
                     `4` = phyKurt),
              tcl = -0.1)
    mtext('Kurtosis', side = 2, line = 1.25)
}


close.screen(all.screens = TRUE)

dev.off()
```

We can also explore how well the $f(\beta_k)$ fit at different taxonomic levels in the script `analysis/pbeta_diffK.R` reproduced below:

```r
# **script to compare within clade volatility distributions at different taxonomic levels**

library(socorro)

# source needed functions
R.utils::sourceDirectory('R', modifiedOnly = FALSE)

load('data/pbdb_sstat_objects.RData')


#' @description function to plot f(beta) distribution
#' @param obj the sstat object
#' @param thrCol color for plotting of theoretical curve

fbetaPlot <- function(obj, thrCol = 'red', ...) {
    betaCDF <- simpECDF(obj$beta, complement = TRUE)
    plot(betaCDF, ylim = c(0, 1.025),
         log = 'x', xaxt = 'n', yaxt = 'n',
```

```r
        xlab = expression(beta), ...)

    logAxis(1, expLab = TRUE)

    curve(pgamma(x, obj$gam.par[1], obj$gam.par[2],
                 lower.tail = FALSE),
          col = thrCol, lwd = 2, add = TRUE)

}


# the plotting
pdf('ms/figSupp_fbeta_allTaxa.pdf', width = 9, height = 3)

split.screen(c(1, 4))

screen(1, new = FALSE)
par(mar = c(0.3, 0.3, 1.5, 0.3), oma = c(2.5, 2.5, 0, 0),
    mgp = c(2, 0.5, 0))
fbetaPlot(sstatPBDBfam3TP)
axis(2)
mtext('Families', side = 3, line = 0.5)

screen(2, new = FALSE)
par(mar = c(0.3, 0.3, 1.5, 0.3), oma = c(2.5, 2.5, 0, 0),
    mgp = c(2, 0.5, 0))
fbetaPlot(sstatPBDBOrd)
mtext('Oders', side = 3, line = 0.5)

screen(3, new = FALSE)
par(mar = c(0.3, 0.3, 1.5, 0.3), oma = c(2.5, 2.5, 0, 0),
    mgp = c(2, 0.5, 0))
fbetaPlot(sstatPBDBCls)
mtext('Classes', side = 3, line = 0.5)

screen(4, new = FALSE)
par(mar = c(0.3, 0.3, 1.5, 0.3), oma = c(2.5, 2.5, 0, 0),
    mgp = c(2, 0.5, 0))
fbetaPlot(sstatPBDBPhy)
mtext('Phyla', side = 3, line = 0.5)

mtext(expression(beta), side = 1, outer = TRUE, line = 1.25)
mtext('Cumulative density', side = 2, outer = TRUE, line = 1.25)

close.screen(all.screens = TRUE)
dev.off()
```

Part of our argument about the failure of superstatistics at higher taxonomic levels is that these higher taxa aggregate increasingly disparate subtaxa. To investigate this idea we look at the number of ecospace hypercubes represented by the average taxon at each taxonomic level in the script `analysis/pbdb_ecoEvoSpace.R` shown here:

```r
# **a script to evaluate hour occupancy of eco-evolutionary space changes
# across taxonomy**
```

```r
library(socorro)

pbdbDat <- read.csv('data/pbdb_data.csv', as.is = TRUE)

# extract only the eco/evo/life history data and remove duplicates
# `taxon_environment`, `reproduction`, `ontogeny`
eeSpaceDat <- pbdbDat[, c('phylum', 'class', 'order', 'family', 'otu',
                           'taxon_environment', 'motility', 'life_habit',
                           'vision', 'diet', 'reproduction', 'ontogeny')]
eeSpaceDat <- eeSpaceDat[!duplicated(eeSpaceDat), ]

# remove entries that are all missing
eeSpaceDat <- eeSpaceDat[rowSums(eeSpaceDat[, -(1:5)] != '') != 0, ]


#' function to determine how many eco-evo hypercubes are occupied by each taxonomic level
#' @param tax the taxonomic unit to consider
#' @param eeDat a data.frame containing eco-evo data
eeOcc <- function(tax, eeDat) {
    sapply(split(eeDat[tax != '', ], tax[tax != '']),
           function(x) sum(!duplicated(x)))
}

#' bootstraps ee space occupancy
#' @param x the vector of niche occupancies
#' @param B number of bootrap replicates
#' @param fun the function to apply to each replicate
eeOccBoot <- function(x, B, fun) {
    replicate(B, fun(sample(x, length(x), replace = TRUE)))
}


# calculate eco-evolutionary space occupancy of each taxonomic level
famEE <- eeOccBoot(eeOcc(eeSpaceDat$family, eeSpaceDat[, -(1:5)]), 500, mean)
ordEE <- eeOccBoot(eeOcc(eeSpaceDat$order, eeSpaceDat[, -(1:5)]), 500, mean)
clsEE <- eeOccBoot(eeOcc(eeSpaceDat$class, eeSpaceDat[, -(1:5)]), 500, mean)
phyEE <- eeOccBoot(eeOcc(eeSpaceDat$phylum, eeSpaceDat[, -(1:5)]), 500, mean)


# plotting
pdf('ms/figSupp_eeSpaceOcc.pdf', width = 4, height = 3.5)

par(mar = c(3, 3, 0, 0) + 0.5, mgp = c(2, 0.75, 0))
plot(1:4, ylim = c(1, 100), type = 'n', log = 'y', yaxt = 'n', xaxt = 'n',
     xlab = 'Taxonomic level', ylab = 'Number of Bambach guilds')
axis(1, at = 1:4, labels = c('Families', 'Orders', 'Classes', 'Phyla'))
logAxis(2)
segments(x0 = 1:4, y0 = c(min(famEE), min(ordEE), min(clsEE), min(phyEE)),
         y1 = c(max(famEE), max(ordEE), max(clsEE), max(phyEE)), lwd = 2)
points(1:4, c(mean(famEE), mean(ordEE), mean(clsEE), mean(phyEE)), pch = 16, cex = 1.2)

dev.off()
```

## A4 Helper functions

All the above analyses make use of helpful functions in the `R` directory. We reproduce those functions below:

```r
#' helper function to calculate corrected flux
#' @param x the matrix of corrected diversities over which to calculate fluxes

calcFlux <- function(x) {
    apply(x, 2, function(X) {
        flux <- diff(c(0, X))
        return(flux[flux != 0])
    })
}
```

```r
gammaLS <- function(data,comp=FALSE) {
    par.init <- c(mean(data)^2,mean(data))/var(data)
    optim(par.init,gamma.ss,data=data,comp=comp)
}

gamma.ss <- function(pars,data,comp) {
    shape <- pars[1]
    rate <- pars[2]
    tabz <- table(data)
    xval <- as.numeric(names(tabz))
    yval <- cumsum(as.numeric(tabz))/sum(tabz)
    if(comp) {
        yval <- 1 - yval
        yval <- c(1,yval[-length(yval)])
        lower <- FALSE
    } else {
        lower <- TRUE
    }
    difz <- pgamma(xval,shape=shape,rate=rate,lower.tail=lower) - yval
    sum(difz^2)
}
```

```r
#' @description function to produce a matrix of time by taxa with cells of corrected diversity
#' @param rawDiv the raw diversity of each taxon in each time interval
#' @param t3stat the 3 timer stat for each diversity record
#' @param pub the number of publications associated with each diversity record
#' @param taxa the taxon names for each diversity record
#' @param tbin the time interval of each diversity record
#' @param tbinTime times associated with each `tbin`
#' @param minPub minimum number of publications for inclusion in regression analysis
#' @param plotit logical, should plot of taxon richness versus number of publications be made
#' @return a matrix with rows corresponding to time intervals and columns to the given taxa
#' each cell in the matrix represents corrected taxon richness


make3TPub <- function(rawDiv,  t3stat,  pub,  taxa,  tbin,  tbinTime,
                      minPub = 10,  plotit = FALSE) {
    # put data together so can be universally manipulated
    x <- data.frame(rawDiv = rawDiv, t3stat = t3stat, pub = pub, taxa = taxa, tbin = tbin)
    x$tbin <- as.character(x$tbin)
    x$taxa <- as.character(x$taxa)
```

```r
    x <- x[!is.na(t3stat) & pub >=  minPub, ]

    tbinTime <- tbinTime[names(tbinTime) %in% x$tbin]

    # 3-timer correction
    t3cor <- x$rawDiv/x$t3stat

    # publication correction
    logPub <- log(x$pub)
    pubLM <- lm(log(t3cor)~logPub)
    pbdbPubLM <<- pubLM # save regression to global env

    pubResid <- exp(pubLM$residuals)

    # plot so you can verify cuttoff etc.
    if(plotit) {
        plot(log(x$pub), log(t3cor),
             xlab = 'log(Number of publications)',
             ylab = 'log(3T-corrected number of genera)')
        abline(pubLM, col = 'red')
    }

    tbinTaxa <- socorro::tidy2mat(x$tbin, x$taxa, pubResid)

    return(tbinTaxa[names(sort(tbinTime, decreasing = TRUE)), ])
}
```

```r
normLS <- function(data,comp=FALSE) {
    par.init <- c(mean(data),sd(data))
    optim(par.init,norm.ss,data=data,comp=comp)
}

norm.ss <- function(pars,data,comp) {
    mean <- pars[1]
    sd <- pars[2]
    tabz <- table(data)
    xval <- as.numeric(names(tabz))
    yval <- cumsum(as.numeric(tabz))/sum(tabz)
    if(comp) {
        yval <- 1 - yval
        yval <- c(1,yval[-length(yval)])
        lower <- FALSE
    } else {
        lower <- TRUE
    }
    difz <- pnorm(xval,mean=mean,sd=sd,lower.tail=lower) - yval
    sum(difz^2)
}
```

```r
# pdf for P(x) with f(beat) ~ Gamma
#' @param x diversity fluctuation value
#' @param shape the shape parameter of the gamma distribution
#' @param rate the rate parameter  of the gamma distribution
```

```r
Px.gam <- PxGam <- function(x, shape, rate) {
    scale <- 1 / rate
    n <- 2 * shape
    b0 <- scale * shape

    t1 <- gamma((n+1) / 2) / gamma(n / 2)
    t2 <- sqrt(b0 / (pi * n))
    t3 <- (1 + (b0 * x^2) / n)^-((n + 1) / 2)

    t1 * t2 * t3
}

# cdf for P(x) with f(beat) ~ Gamma
#' @param x diversity fluctuation value
#' @param shape the shape parameter of the gamma distribution
#' @param rate the rate parameter  of the gamma distribution
#' @param comp logical, whether to compute the complement or not (`comp = TRUE` is
#' equivilant to `lower.tail = FALSE` for typical `p` functions [e.g. `pnorm`])

PPx.gam <- PPxGam <- function(x, shape, rate, comp=TRUE) {
    if(length(x) == 1) {
        intgral <- integrate(PxGam, 0, x, shape = shape, rate = rate)
        if(intgral$message != 'OK') print(intrgral$message)
        val <- intgral$value

        if(comp) {
            return(1 - 2 * val)
        } else {
            return(2 * val)
        }

    } else {
        # recursive handeling for multiple `x` values
        return(sapply(x, function(X) PPxGam(X, shape, rate, comp)))
    }
}
```

```r
#' @description gives the log likelihood function under sstat model
#' @param par the parameter values
#' @param dat the data

sstatLL <- function(par, dat) {
    -sum(log(Px.gam(dat,par[1], par[2])))
}


#' @description finds the maximum likelihood estimate of the superstats model
#' @param dat the data to fit

sstatMLE <- function(dat) {
    optim(c(0.55, 0.17), sstatLL, method = 'BFGS', hessian = TRUE,
          dat = dat)
}
```

```r
#' @description bootstrap likelihood for super stats model
#' @param x the `sstat` object
#' @param B the number of boostrap replicates
#' @param useAll logical, whether all orders, or only those with the minimum number of
#' occurences as specified
#' in `make3TPub` argument `minPub` should be used

bootMLE.sstat <- function(x, B = 1000, useAll = FALSE) {
    if(useAll) {
        theseDat <- x$Px.raw
    } else {
        theseDat <- x$Px.sub
    }

    boots <- replicate(B, {
        subDat <- sapply(theseDat, sample, size = 1)

        thisMLE <- try(sstatMLE(subDat), silent = TRUE)

        if(class(thisMLE) !=  'try-error') {
            if(thisMLE$convergence !=  0) {
                out <- rep(NA, 2)
            } else {
                out <- thisMLE$par
            }
        } else {
            out <- rep(NA, 2)
        }
        out
    })

    sstatOut <- rbind(quantile(boots[1, ], c(0.025, 0.975), na.rm = TRUE),
                      quantile(boots[2, ], c(0.025, 0.975), na.rm = TRUE))
    rownames(sstatOut) <- c('shape', 'rate')

    return(list(sstat = sstatOut))
}


#' @description logLik for sstat class
#' @param x the `sstat` object
#' @param fitted logical, was the model fitted by max likelihood or computed from first
#' principles
#' @param useAll logical, should all data be used, or only those taxa that have greater
#' than `minN` occurrences
#' as specified in `sstatComp`

logLik.sstat <- function(x, fitted = TRUE, useAll = FALSE) {
    if(useAll) {
        theseDat <- unlist(x$Px.raw)
    } else {
        theseDat <- unlist(x$Px.sub)
    }
```

```r
    lik <- sum(log(x$Px(theseDat)))

    if(fitted) {
        attr(lik, 'df') <- 2
    } else {
        attr(lik, 'df') <- 0
    }

    class(lik) <- 'logLik'

    return(lik)
}
```

```r
#' @description plot method for sstat class
#' @param x the `sstat` object
#' @param sstatCol color for super stats fit
#' @param normCol color for Gaussian fit
#' @param showNorm logical, should Gaussian fit be shown
#' @param addLegend logical, should legend be added
#' @param ... other parameters passed to `plot.default`

plot.sstat <- function(x, sstatCol = 'red', normCol = 'blue',
                       showNorm = TRUE, addLegend = TRUE, ...) {
    thisECDF <- socorro::simpECDF(abs(unlist(x$Px.sub)), complement = TRUE)

    # helper function to deal with optional axis arguments
    .axissetup <- function(side) {
        if(sprintf('%saxt', side) %in% names(pargs)) {
            if(pargs[[sprintf('%saxt', side)]] == 'n') {
                assign(sprintf('%saxfun', side), function(...) {}, pos = 1)
            } else {
                if(side %in% pargs$log) {
                    assign(sprintf('%saxfun', side), socorro::logAxis, pos = 1)
                } else {
                    assign(sprintf('%saxfun', side), axis, pos = 1)
                }
            }
        } else {
            if(side %in% pargs$log) {
                assign(sprintf('%saxfun', side), socorro::logAxis, pos = 1)
            } else {
                assign(sprintf('%saxfun', side), axis, pos = 1)
            }
        }
    }

    pargs <- list(...)
    if(!('log' %in% names(pargs))) pargs$log <- 'xy'
    if(!('xlab' %in% names(pargs))) pargs$xlab <- '|Fluctuations|'
    if(!('ylab' %in% names(pargs))) pargs$ylab <- 'Cumulative density'
    .axissetup('x')
    .axissetup('y')
```

```r
    pargs$xaxt <- 'n'
    pargs$yaxt <- 'n'

    do.call(plot, c(list(x = thisECDF), pargs))
    xaxfun(1)
    yaxfun(2)

    PPx <- x$PPx
    curve(PPx(x, comp = TRUE), col = sstatCol, lwd = 2, add = TRUE)

    if(showNorm) {
        thisSD <- sd(unlist(x$Px.sub))
        curve(2*pnorm(x, 0, thisSD, lower.tail = FALSE), col = normCol, lwd = 2, add = TRUE)
    }

    if(addLegend) {
        leg <- c('Observed', 'Superstatistics')
        col <- c(par('fg'), sstatCol)
        pch <- c(ifelse('pch' %in% names(list(...)), list(...)$pch, 1), NA)
        pt.lwd <- c(1, NA)
        pt.cex <- c(1, NA)
        lwd <- c(NA, 2)

        if('panel.first' %in% names(list(...))) {
            leg <- c(leg, 'Superstatistics CI')
            col <- c(col, socorro::colAlpha(sstatCol, 0.25))
            pt.lwd <- c(pt.lwd, 1)
            pt.cex <- c(pt.cex, 2)
            lwd <- c(lwd, NA)
            pch <- c(pch, 15)
        }

        if(showNorm) {
            leg <- c(leg, 'Gaussian')
            col <- c(col, normCol)
            pt.lwd <- c(pt.lwd, NA)
            pt.cex <- c(pt.cex, NA)
            lwd <- c(lwd, 2)
            pch <- c(pch, NA)
        }

        extracex <- ifelse('cex' %in% names(list(...)), list(...)$cex, 1)
        legend('bottomleft', legend = leg, col = col, pch = pch, pt.lwd = pt.lwd,
               pt.cex = pt.cex*extracex, lwd = lwd, bty = 'n')
    }
}


#' @description function to add confidence interval polygon from ML analysis
#' @param ci the matrix of CI intervals for the parameter values returned by `bootMLE.sstat`
#' @param fun the CDF function to plug the parameter values into
#' @param ... further arguments passed to `polygon` (e.g. `col`, `boarder`, etc.)
```

```
mlePoly <- function(ci, fun, ...) {
    n <- 50
    x <- seq(par('usr')[1], par('usr')[2], length = n)
    x <- c(x, rev(x))

    if(par('xlog')) x <- 10^x

    y <- c(fun(x[1:n], ci[1, 1], ci[2, 2]), fun(x[(1:n) + n], ci[1, 2], ci[2, 1]))

    polygon(x = x, y = y, ...)
}
```

```
sstatComp <- function(grp.data,minN=15,xlab="Absolute Fluctuation",
                      ylab="Cumulative Density",leg=TRUE,plotit=TRUE) {
    these2use <- sapply(grp.data,length) >= minN
    p2use <- grp.data[these2use]

    cat("computing Gaussian fit for p_k(x|sigma) \n")
    pk.par <- sapply(p2use,function(x) unlist(normLS(x)[c("par","value")]))
    pk.par <- t(pk.par)
    colnames(pk.par) <- c("mu","sig","ss")

    cat("re-centering \n")
    for(i in 1:length(p2use)) {
        p2use[[i]] <- p2use[[i]] - pk.par[i,"mu"]
    }

    cat("computing f(beta) \n")
    f.beta.par <- gammaLS(1/(pk.par[,"sig"])^2)$par
    fuent.par <- c(n=2*f.beta.par[1],b0=f.beta.par[1]*f.beta.par[2])

    cat("computing P(x) \n")
    this.Px <- function(x) Px.gam(x,f.beta.par[1],f.beta.par[2])
    this.PPx <- function(x,comp=TRUE) PPxGam(x,f.beta.par[1],f.beta.par[2],comp)

    out <- list(gam.par=f.beta.par,sspar=fuent.par,beta=1/(pk.par[,"sig"])^2,
                sumSq=pk.par[,"ss"],minN=minN,raw.pk=p2use,
                Px.raw=grp.data,Px.sub=p2use,incld=these2use,Px=this.Px,PPx=this.PPx)

    class(out) <- "sstat"

    if(plotit) plot(out)

    return(out)
}
```
